# Supplementary material for: Spinning particles in general relativity: Momentum-velocity relation for the Mathisson-Pirani spin condition
Source: arXiv:1712.07281 ancillary file (2018-05-30)
Supplement: Supplementary file 1 [file AdditionalPlots.pdf]

# Additional plots

## 1 - Limit M=0: Helical motions in flat spacetime

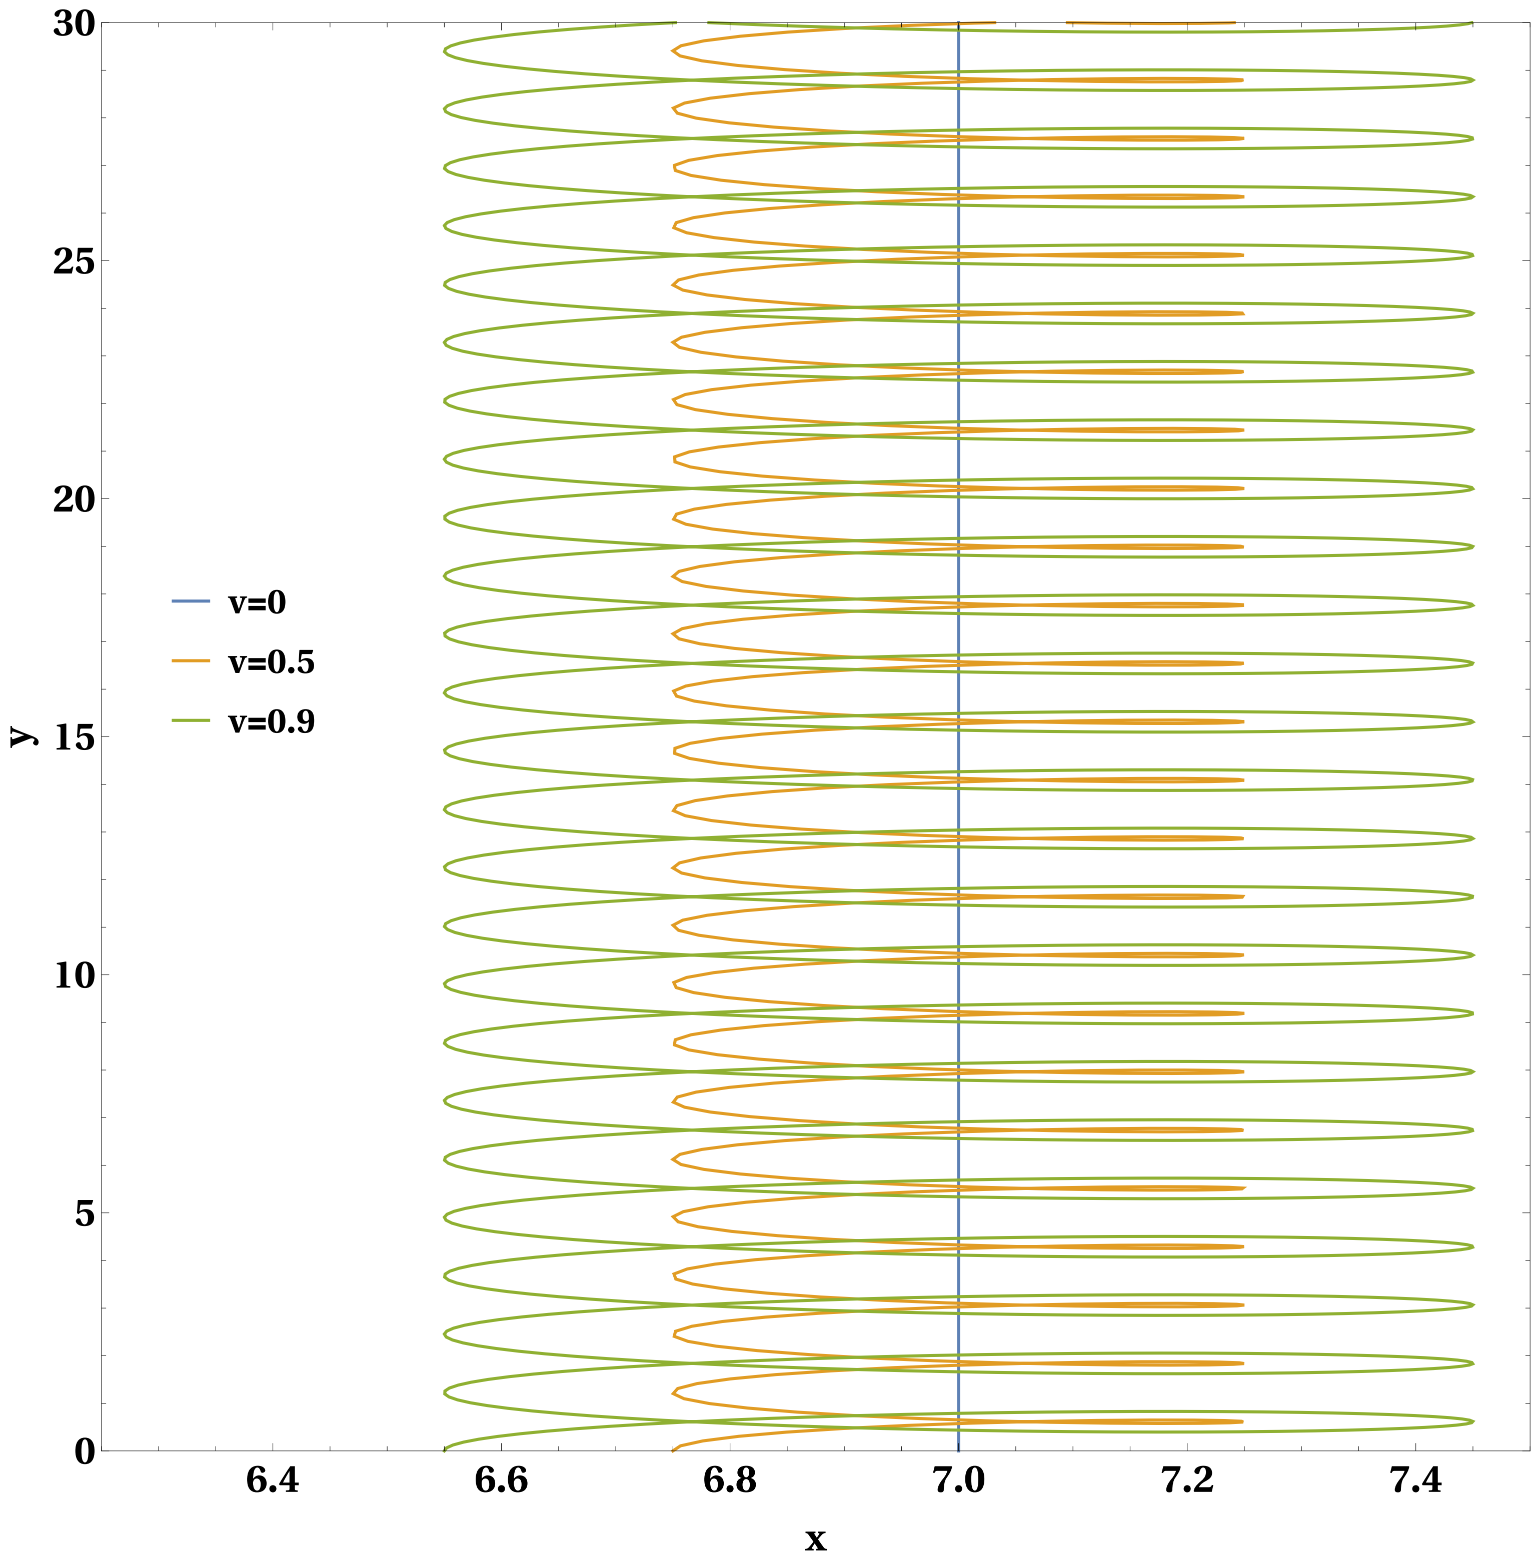


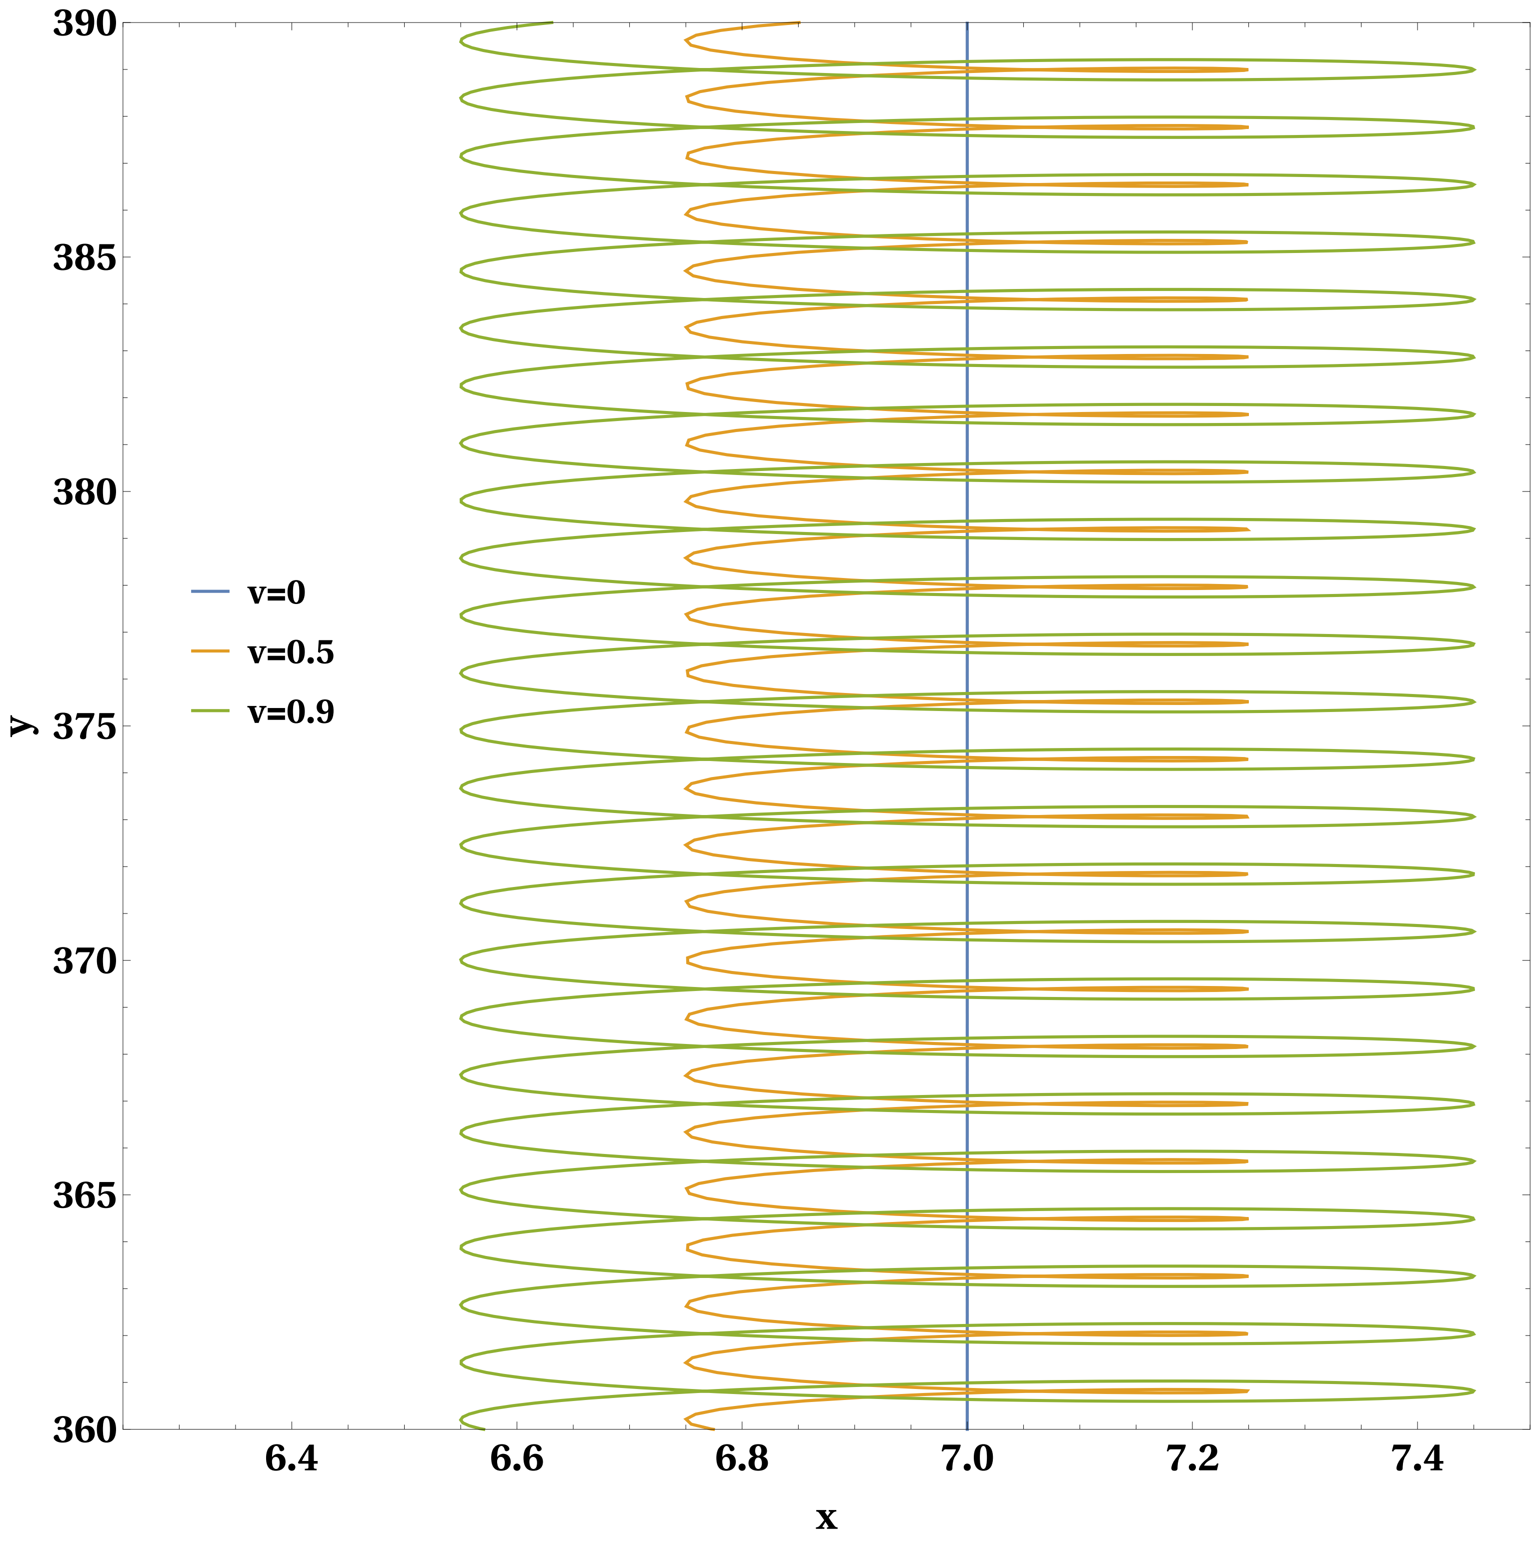

## 2 - Full plot in Fig. 6 -- Circular orbit in Schwarzschild spacetime with radius r=30M, plus the corresponding helical representations for v=0.5 and v=0.9.

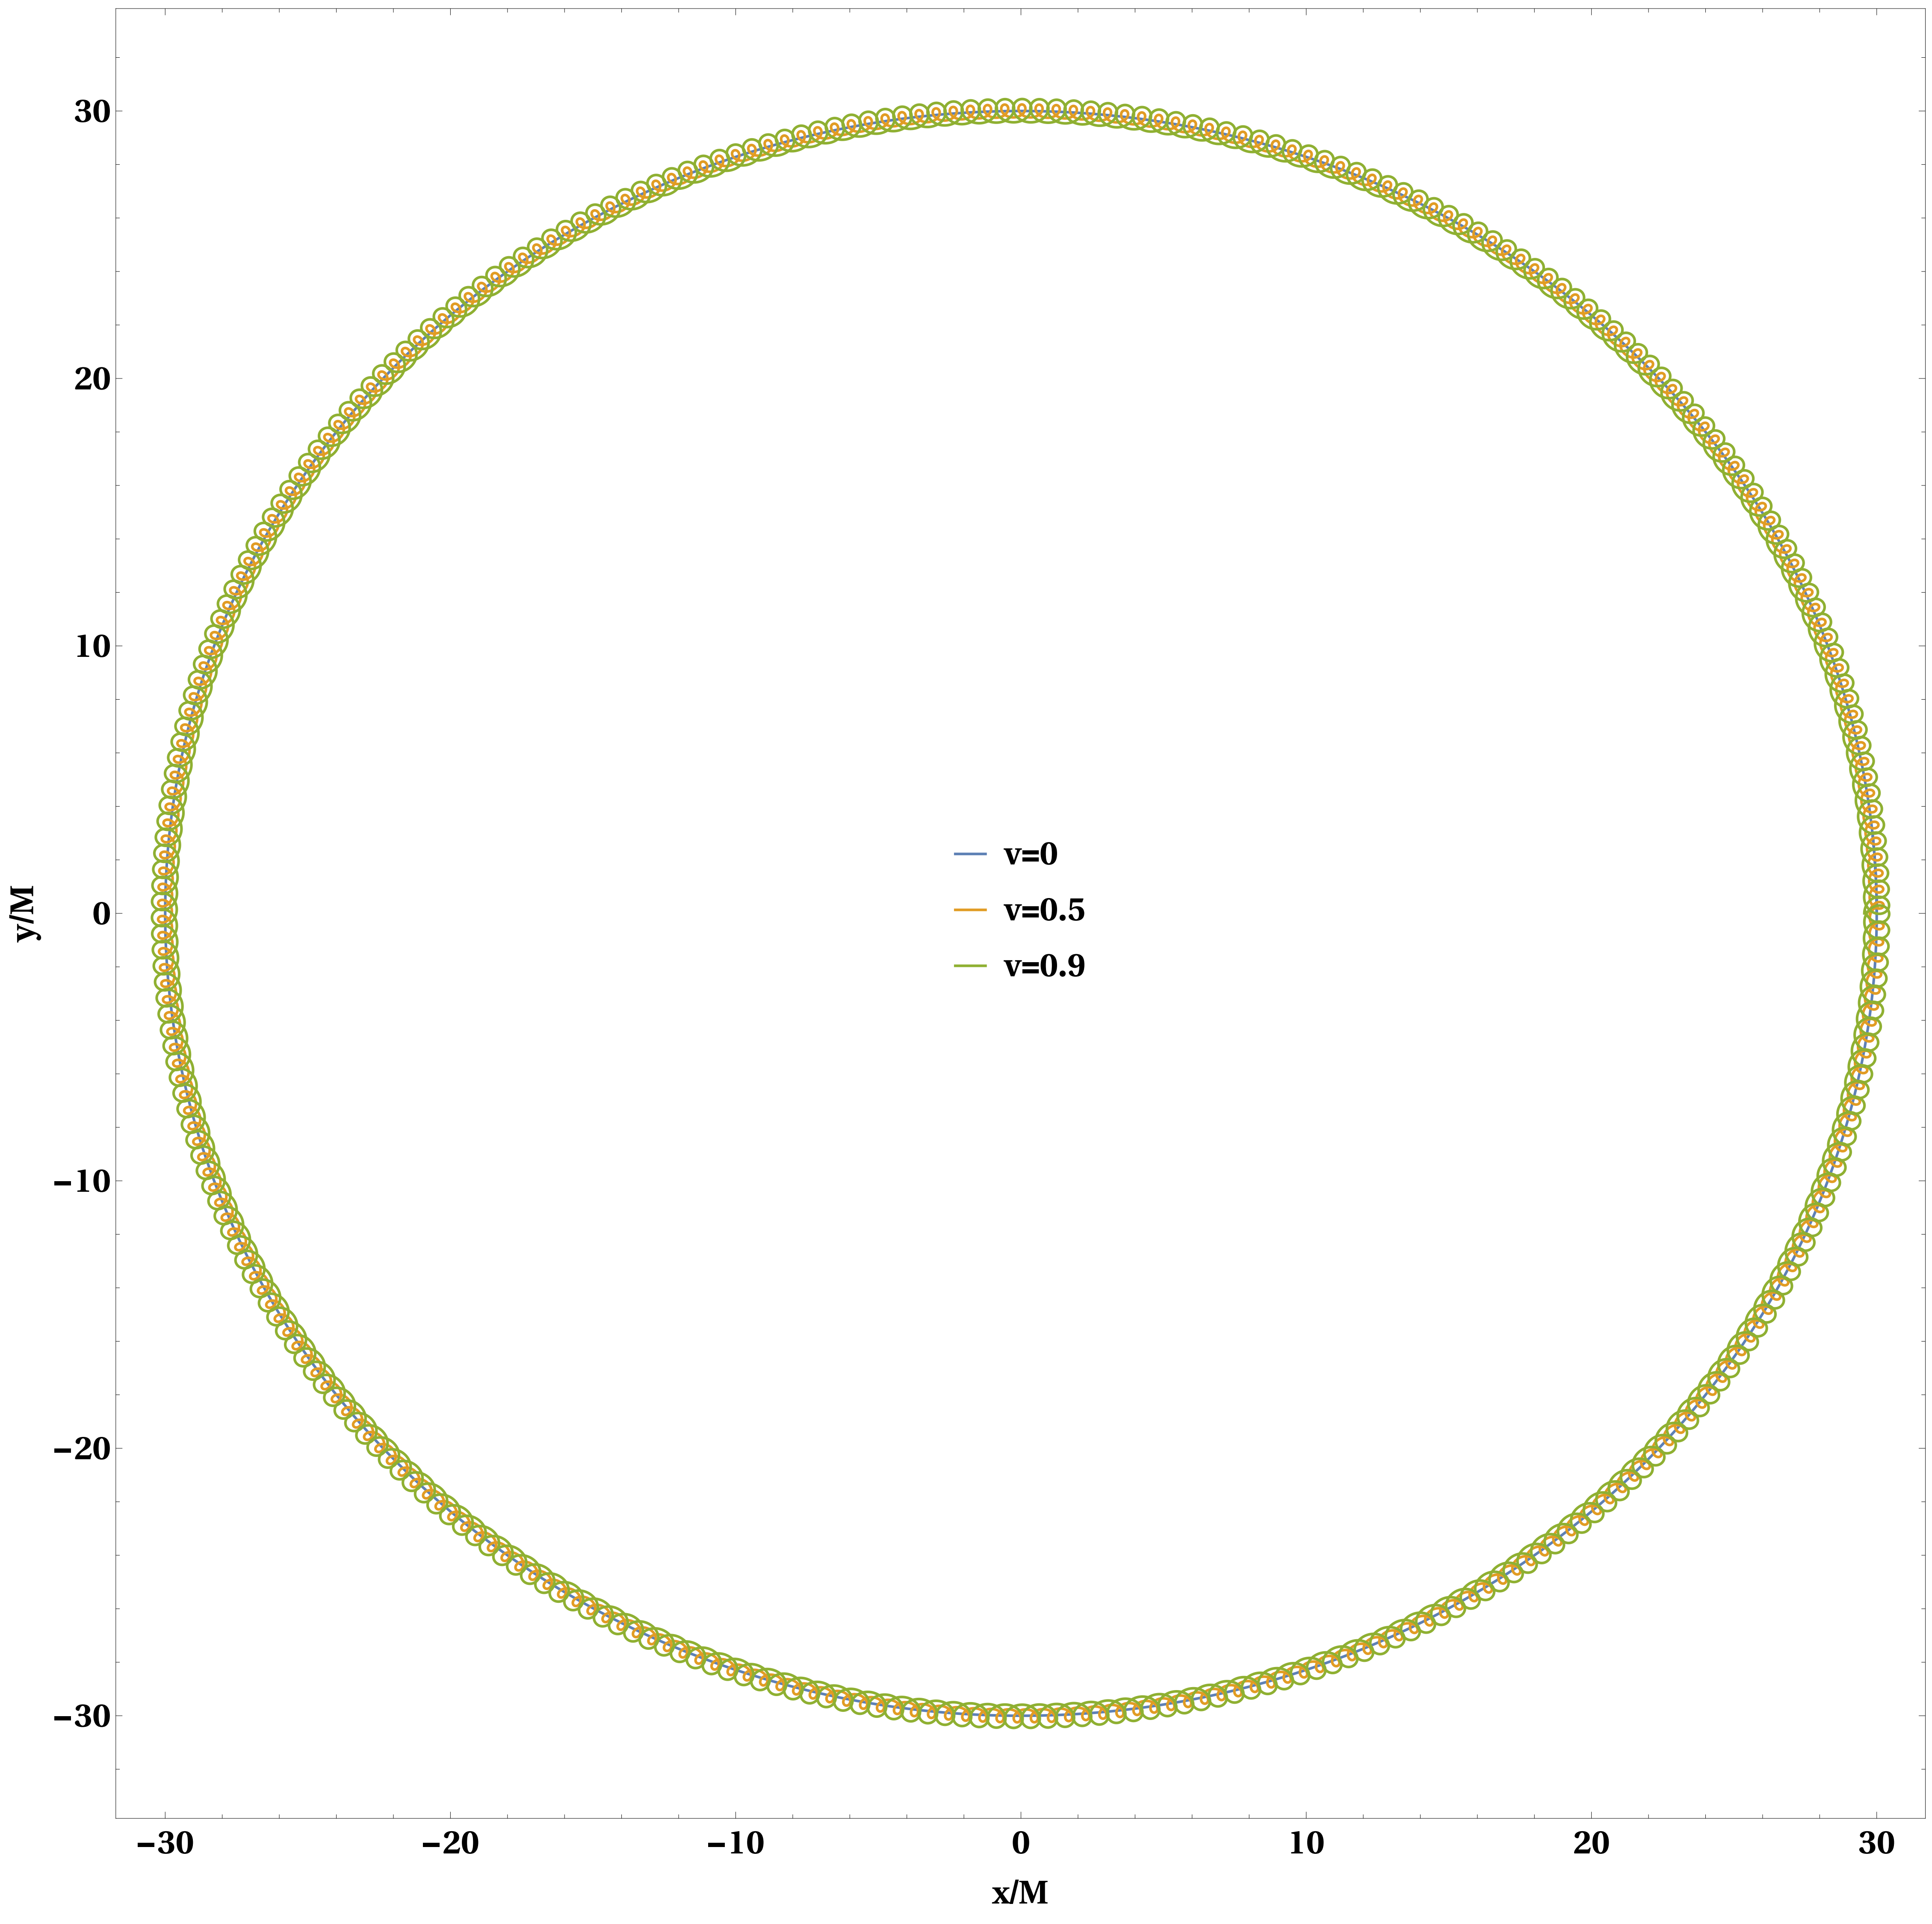

## 3 - Plot analogous to that in Fig. 5, but with with initial shifts of the helices (relative to non-helical centroid) pointing inwards

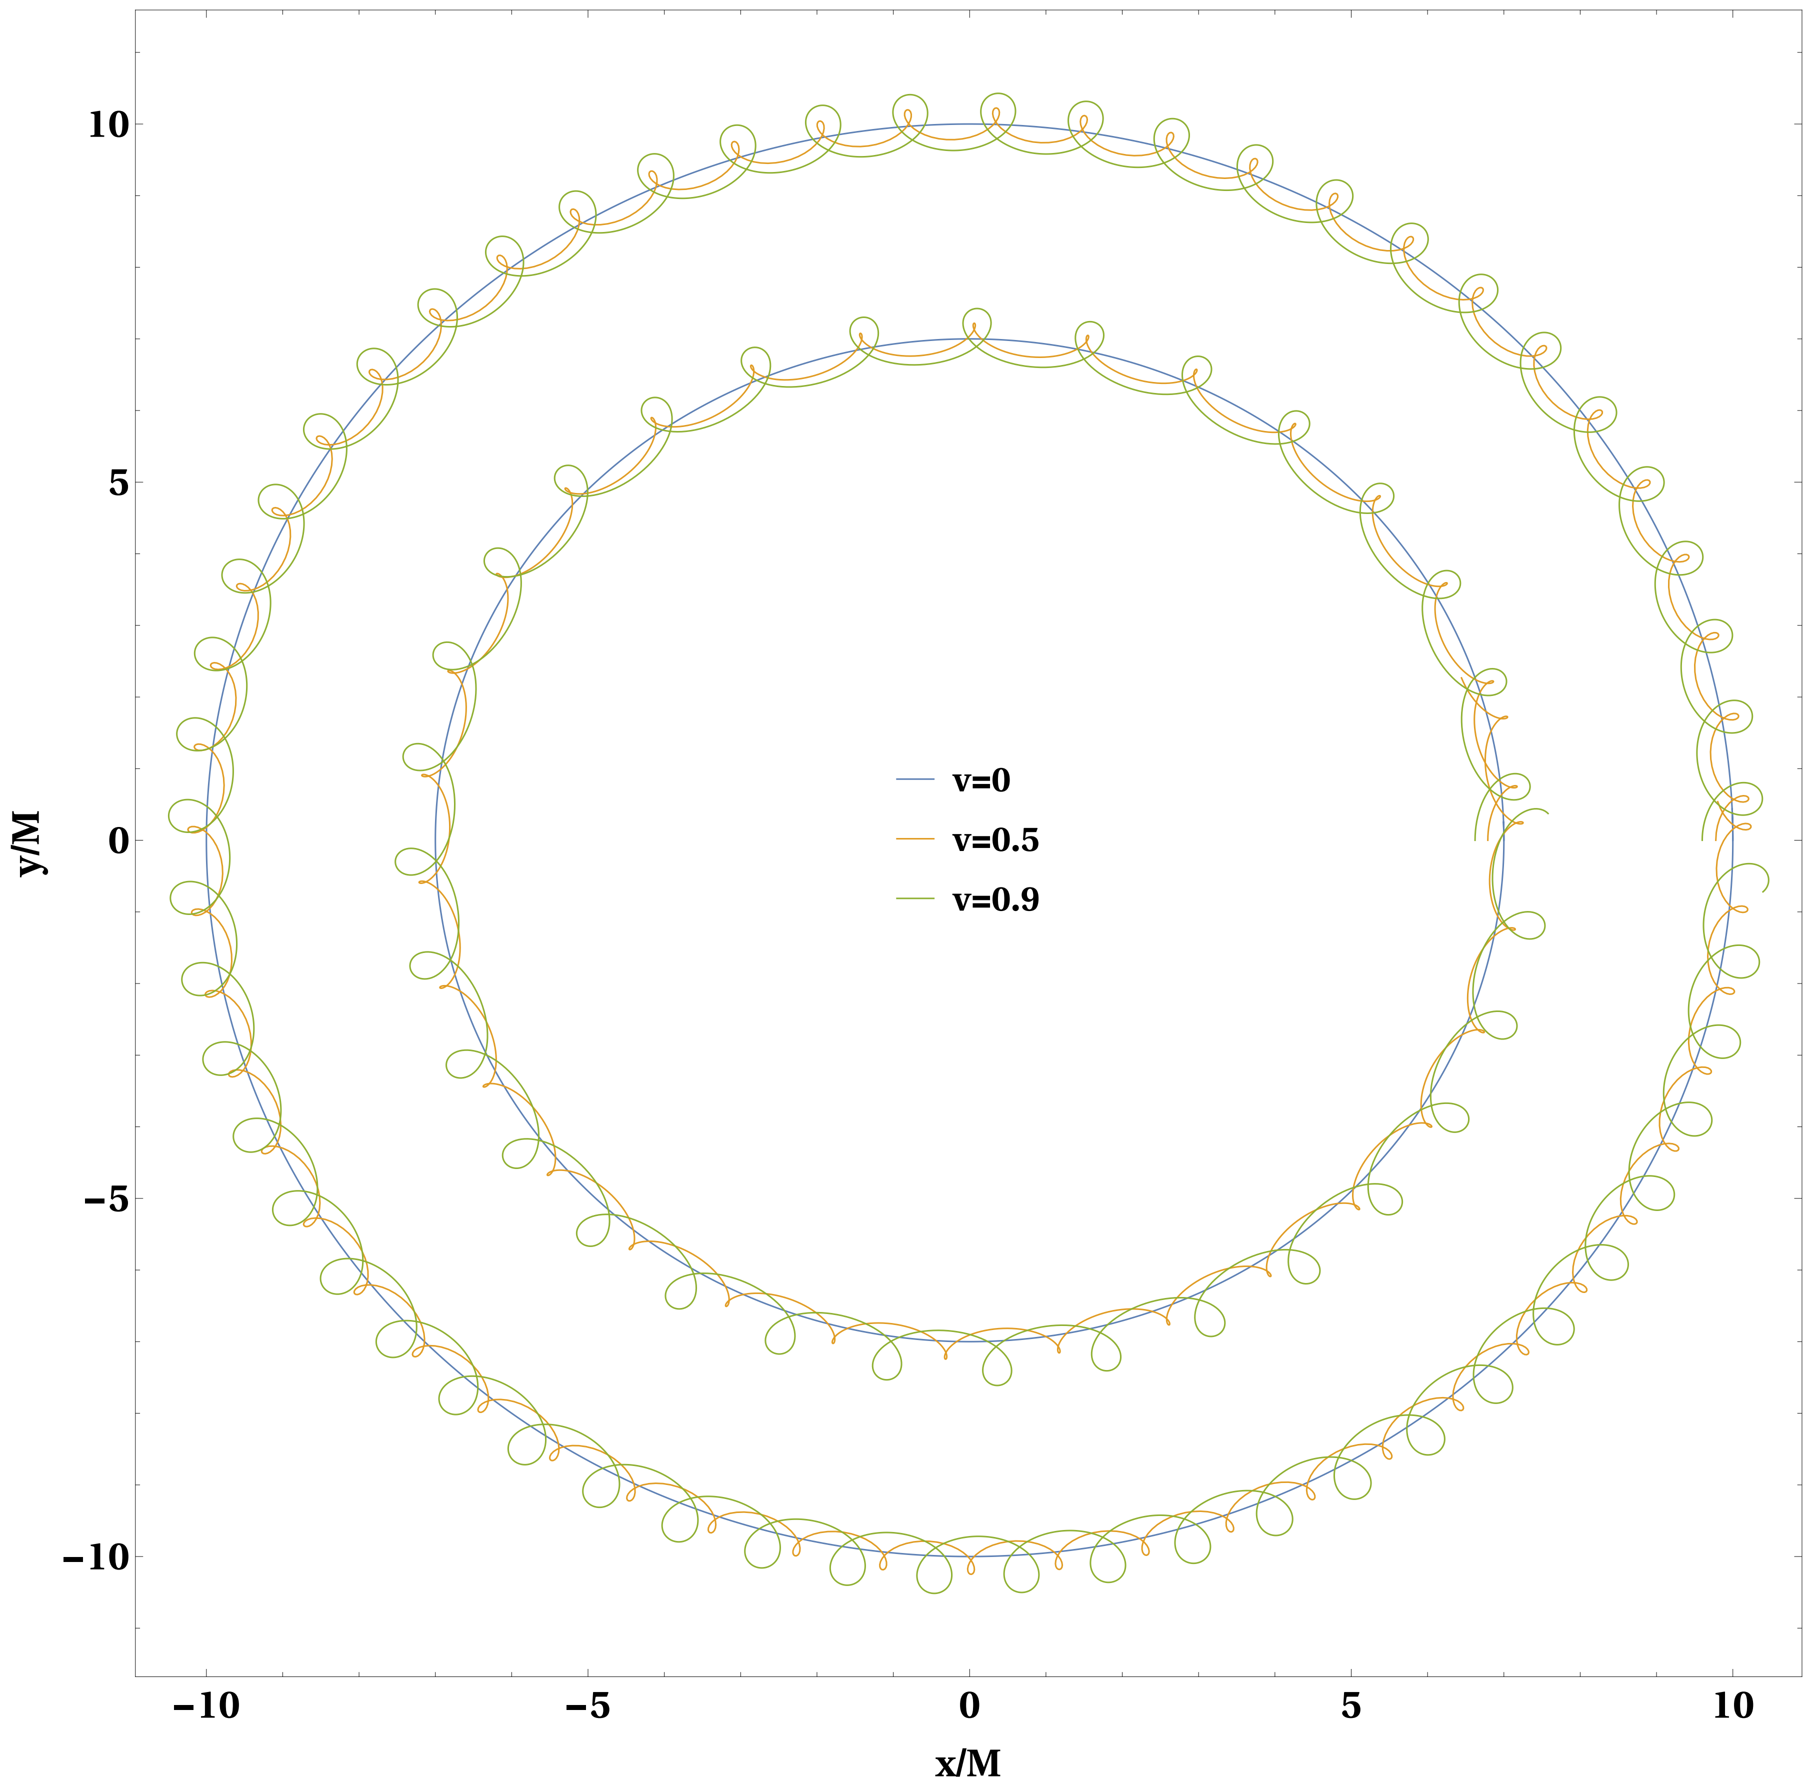


This is set up by choosing $v^{\alpha}|_{\text{in}}$ along the positive $\phi$ direction, i.e., choosing the plus sign in Eq. (69) and the minus sign in Eq. (71) (notice that in Fig. 5, in turn, it is set in the negative $\phi$ direction, leading to an outwards initial shift).

## 4- Several laps plot (outwards initial shift) - continuation of the simulation in Fig. 5

First 10 laps of the fiducial circular orbits, and their corresponding helical representations (v=0.5 and v=0.9), for two values of the radius: r=7M and r=10M.

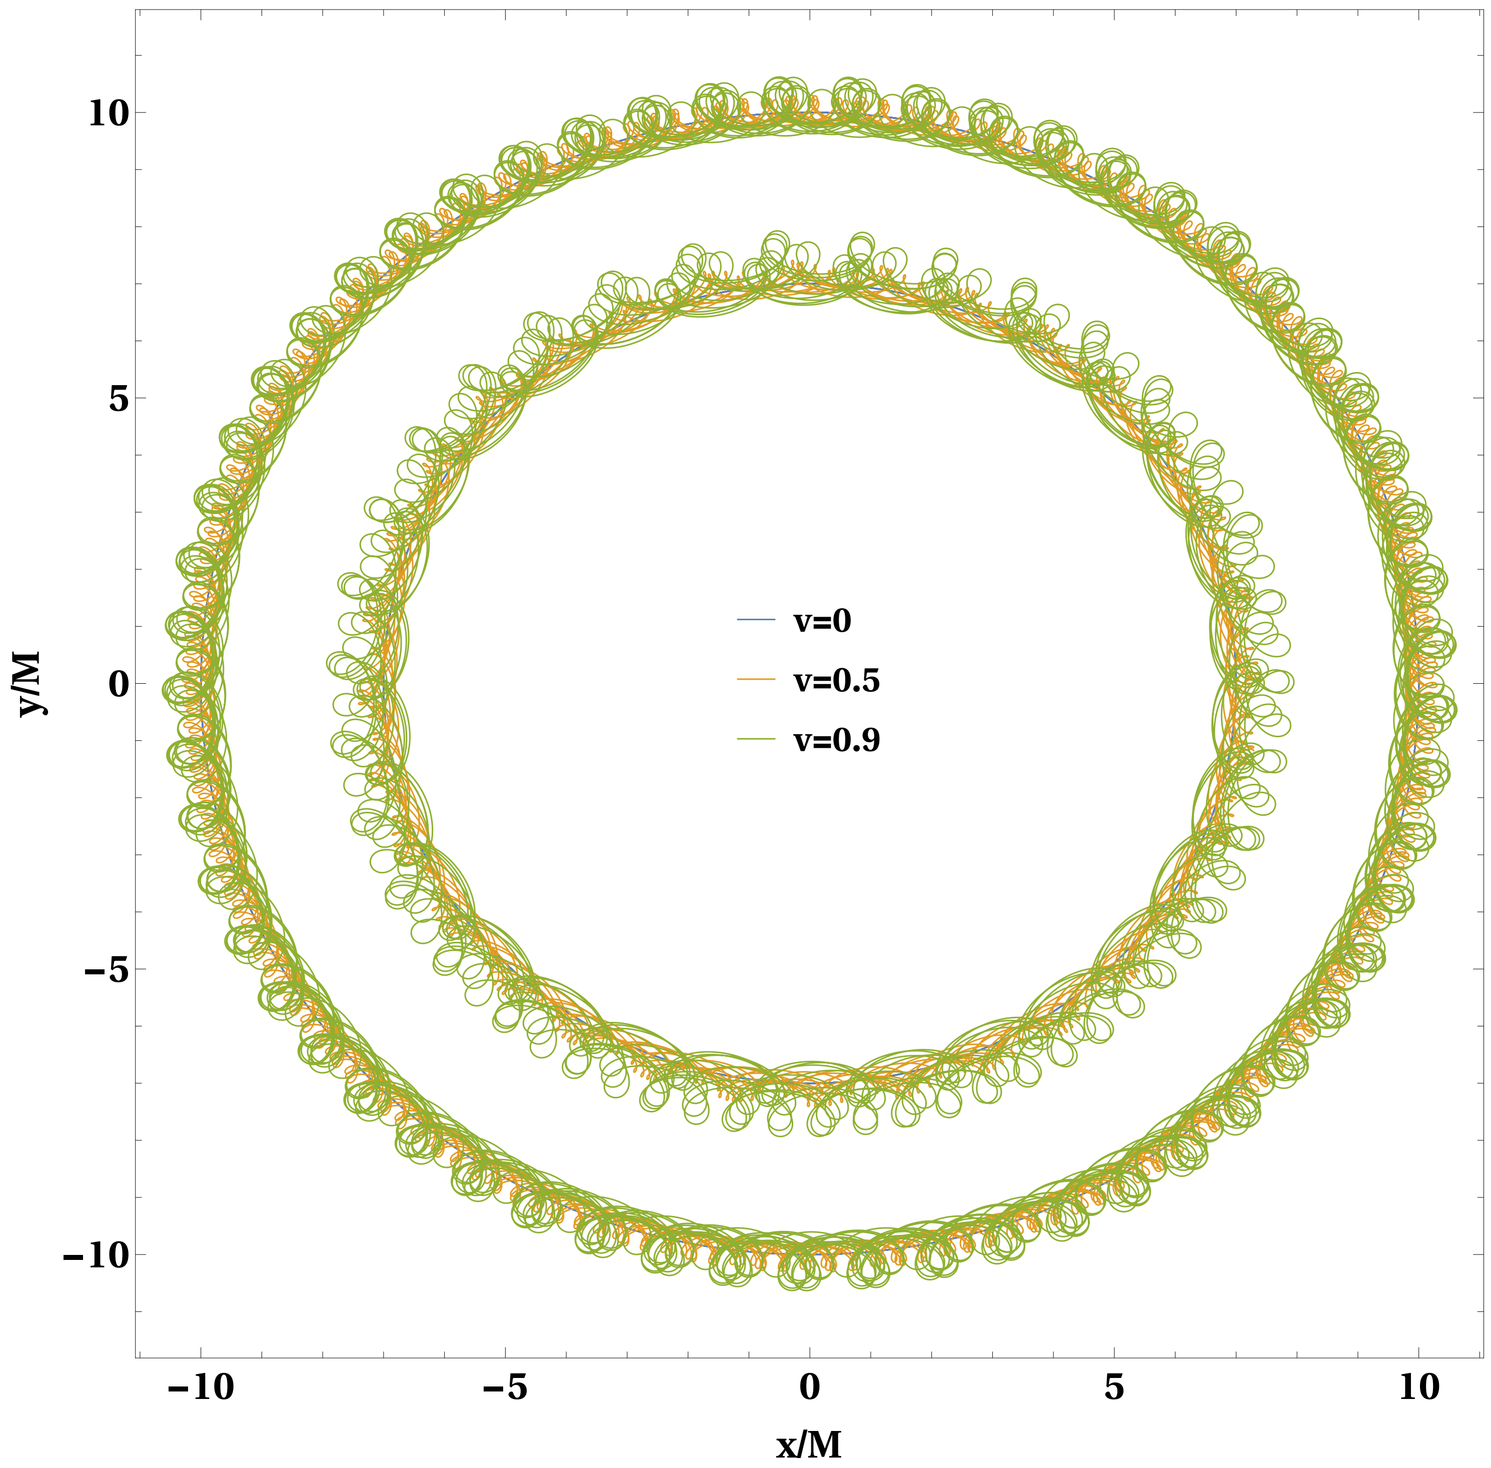


Same plot as above, but showing only the v=0.5 helices:

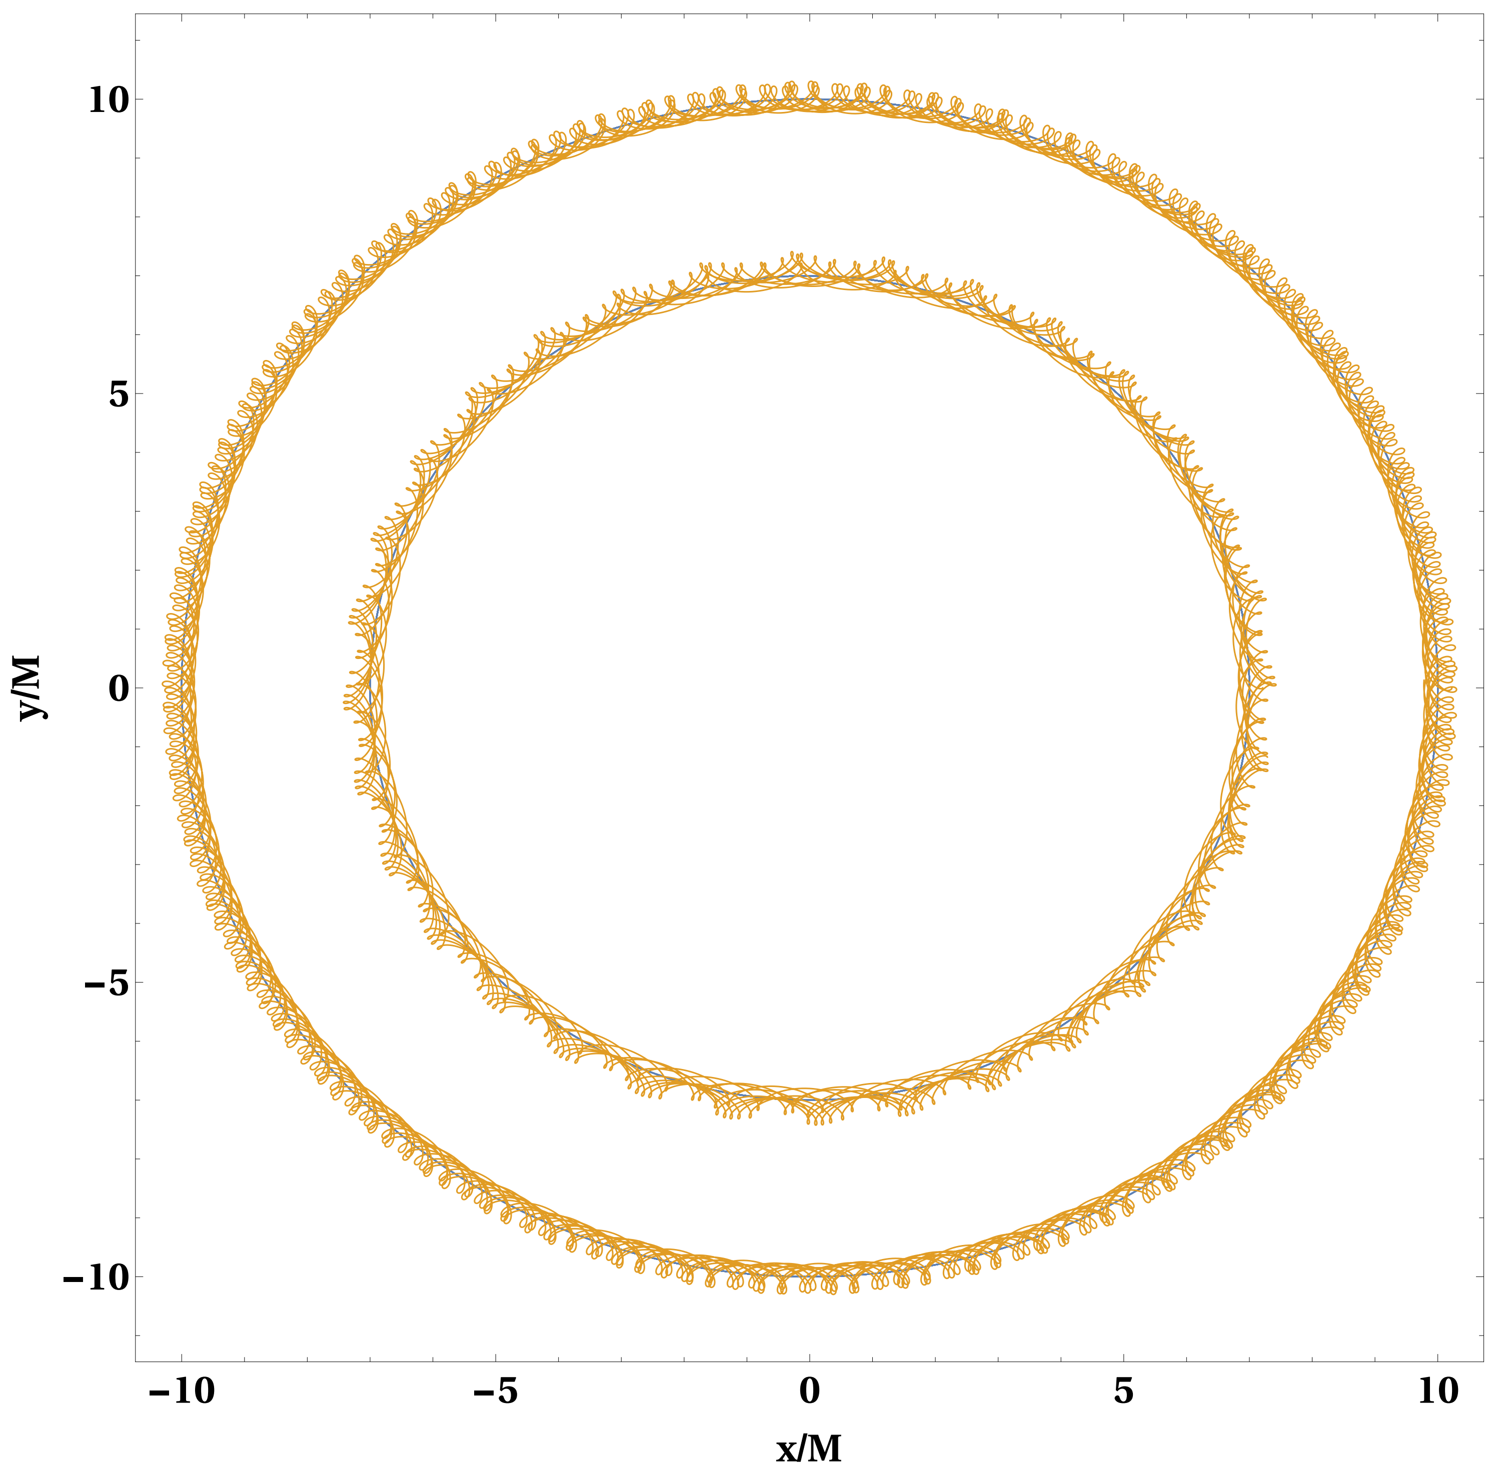


Same plot as above, but showing only the v=0.9 helices:

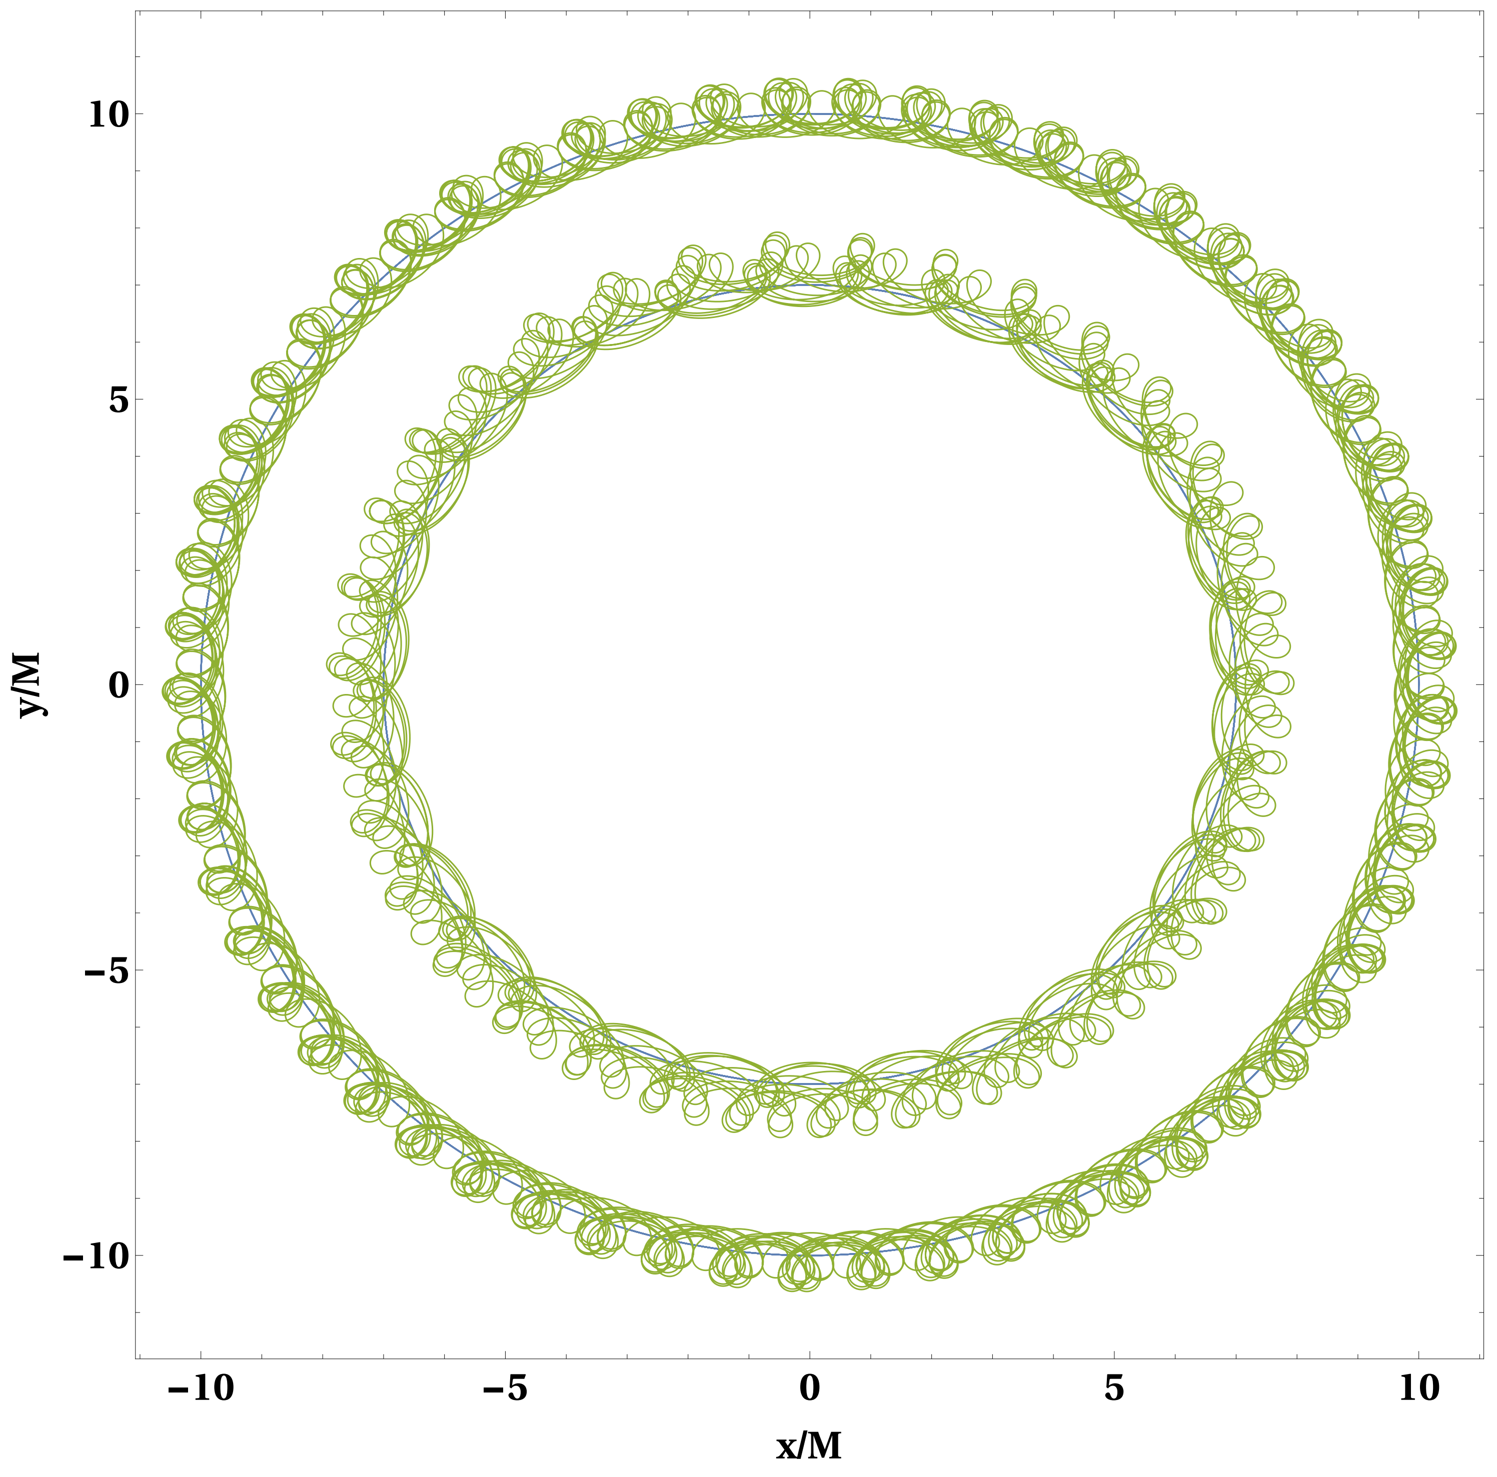


These plots show that for r=10M the different representations of a given body remain, on the whole, remarkably close, sweeping a spatial tube very nearly consistent with the body’s minimal size. For r=7M, however, the trajectories diverge outside such tube.
